# Supplementary material for: Training Deep Neural Networks with Joint Quantization and Pruning of Weights and Activations
Source: arXiv:2110.08271 source file (2021-11-01)
Supplement: Supplementary file 1 [file appendix.tex]

\section{Detailed Experiment Setups}
\label{apn:detailed_exp}



\section{More Experiment Results}
\label{apn:more_exp}

\section{Discussion on Comparing Quantization \& Pruning Performance over Difference Network Structures}
\label{apn:benchmark}



\section{More Samples from Pix2Pix and CycleGAN}
\label{apn:more_demos}
