# Supplementary material for: Training Deep Neural Networks with Joint Quantization and Pruning of Weights and Activations
Source: arXiv:2110.08271 source file (2021-11-01)
Supplement: Supplementary file 4 [file appendix.tex]

\section{Related Work in Details}
\label{apn:related_work}


\textbf{Quantization.} Quantization is the process of quantifying floating
numbers with integer equivalents. Quantization can be applied on both weights
and feature, which can then be used for integer arithmetic. Post-training
quantization operates on a trained network, which is usually more convenient for
deployment but sometimes suffers from accuracy degradation. Quantization-aware
training involves quantization into the training process, which provides better
accuracy but requires to change the original floating point training pipeline.
\citep{n28_krishnamoorthi2018quantizing, n16_wu2020integer} conduct comprehensive
quantization experiments for various applications and proposes best practices
and workflows.

For post-training quantization, \citep{n1_stock2019and} proposes to reduce
reconstruction loss for in-domain inputs which only needs unlabeled data.
\citep{n11_xu2020generative, n12_he2021generative} uses GAN to generate fake data
for post-training quantization. \citep{n15_zhao2019improving} presents a
channel-splitting method to handle outliers during quantization.
\citep{n26_lee2018quantization} also leverages channel-level distribution, but it
conducts experiments on objection detection with  YOLO-v2 \citep{o_yolov2}. For
quantization-aware training, \citep{o_hubara2017quantized} proposes straight
through gradient estimator to calculate gradients for quantization layer.
\citep{n25_jacob2018quantization} inserts simulated quantization operator into an
existing network during training. \citep{n27_yang2019quantization} studies the
relation between quantization  and non-linear activation function.
\citep{n40_choi2016towards} introduces hessian distortion to measure quantization
error. \citep{n41_choi2020universal} applies the idea of randomized lattice
quantization to neural network. \citep{n44_achterhold2018variational} formulates
quantization as a variational inference problem and trains with stochastic
weight and quantize afterwards. \citep{detect_wei2018quantization} conduct
quantization and distillation on tiny object detection networks.
\citep{detect_li2019fully} presents a set of training stabilizing methods for
quantizing object detection networks. \citep{n23_wang2019qgan} designs an EM algorithm
to quantize the weight of a GAN to low bit-width on \citep{o_cifar10, o_celebA}.



\textbf{Pruning.} Sparsity is a long-standing research problem in the neural
network domain \citep{n38_gale2019state, n35_hoefler2021sparsity}, and pruning is
one of the most important technique to obtain sparse neural network by removing
unimportant connections.
\citep{n3_xiao2019autoprune} proposes to prune by optimizing auxiliary
parameters. \citep{n6_venkatesan2020out} uses weight rewinds as a retraining
technique during pruning. \citep{n14_molchanov2019importance} estimates weight
importance to final loss using taylor expansion to guide pruning selection.
\citep{detect_he2017channel} proposes a layer-wise constraint-based channel
pruning method.
\citep{n22_yeom2021pruning} prunes by relevance score from
\citep{o_bach2015pixel}. \citep{n37_frankle2018lottery, n30_evci2020rigging}
claims training network from scratch with pruned structure yields better
performance. \citep{n39_luo2017thinet} presents a method to prune layer-wisely
based on statistics of next layer. \citep{n43_zhao2019variational} designs a
variational inference method to estimate channel importance for pruning.
\citep{n45_zhu2017prune} proposes a stage-wise pruning method with an annealing
process. \citep{n46_chen2018constraint} also designs an annealing pruning
procedure under constrained bayesian optimization perspective.


All of the above methods are for weight pruning, and can be categorized as
structured \citep{o_liu2017learning} and unstructured pruning \citep{o_han2015learning}, while the former one requires to remove a
group of weights together, i.e. channel-wise pruning.
\citep{n29_liu2018rethinking} finds that structured pruning is equivalent to an implicit
neural architecture search but its margin over random pruning is limited. There
are some work connects GAN with sparsity
\citep{n32_mahdizadehaghdam2019sparse, n33_dettmers2019sparse,
n34_zhou2020sparse}, but their major focus is on how to use sparse
regularization to improve generative quality.


\textbf{Joint Quantization and Pruning.} There are not many work that jointly
consider pruning and quantization. \citep{n21_liang2021pruning,
n24_paupamah2020quantisation} claim that they can be studied independently.
\citep{n5_tung2018clip}
focuses on training acceleration for pruning and quantization instead of
accuracy.
\citep{n8_han2015deep, n10_zhao2019focused, n17_yu2020joint} study methods that
prune and quantize weight while ignoring feature. \citep{n17_yu2020joint} also
advices pruning shall happens before quantization but merely from the
quantization error perspective.
\citep{n4_van2020bayesian} presents an integer optimization inspired
method that quantizes weight \& feature, and prunes weight, but it does not
study feature pruning nor does it discloses its implementation.
\citep{detect_tzelepis2019deep} proposes a dynamical clustering based model
compression method with pruning and quantization and conduct experiments on
object detection tasks, but does not report detailed resulting accuracy.



\textbf{Neural Network Compression Toolbox.} There are many open-source or
proprietary neural network compression tools that provide pruning or
quantization functionality. However, as far as our best knowledge, none of them
offer joint pruning \& quantization on both weight and feature. Moreover, many
tools are designed to be heavy and requires developers to write code in a
domain-specific language (DSL), which is highly inflexible.


\citep{t_intel} is one of the most comprehensive tool, which supports both
pruning and quantization, but it does not provide joint-training examples. It
also requires writing complex schedule files in order to train models.
\citep{AiMet} implements a set of pruning and quantization methods separately and
provides few examples. \citep{TorchPruning} only has structured pruning.
\citep{n10_zhao2019focused} provides a joint method implementation, but it only
works on weight and it ships with a set of obscure DSL.
\citep{n18_shah2020kd} includes module-level API on pruning and quantization
individually. \citep{t_xilinx} has a set of layer-level neural network API, which
is more flexible, but it only provides quantization-aware training, and later we
will see our API design is much simpler and versatile. PyTorch
\citep{t_paszke2019pytorch} has built-in support for both functions, but
\citep{QuantizationTorch,PruneTorch} only works on module-level and has limited
support on quantization-aware training \citep{QatTorch}. \citep{TensorRT}
provides post-training quantization only and mainly focuses on its efficient CUDA
inference library. 



\section{Detailed Experiment Setups}
\label{apn:detailed_exp}



\section{More Experiment Results}
\label{apn:more_exp}


\begin{figure}[h]
	\begin{center}
		\scalebox{0.5}{
			\includegraphics{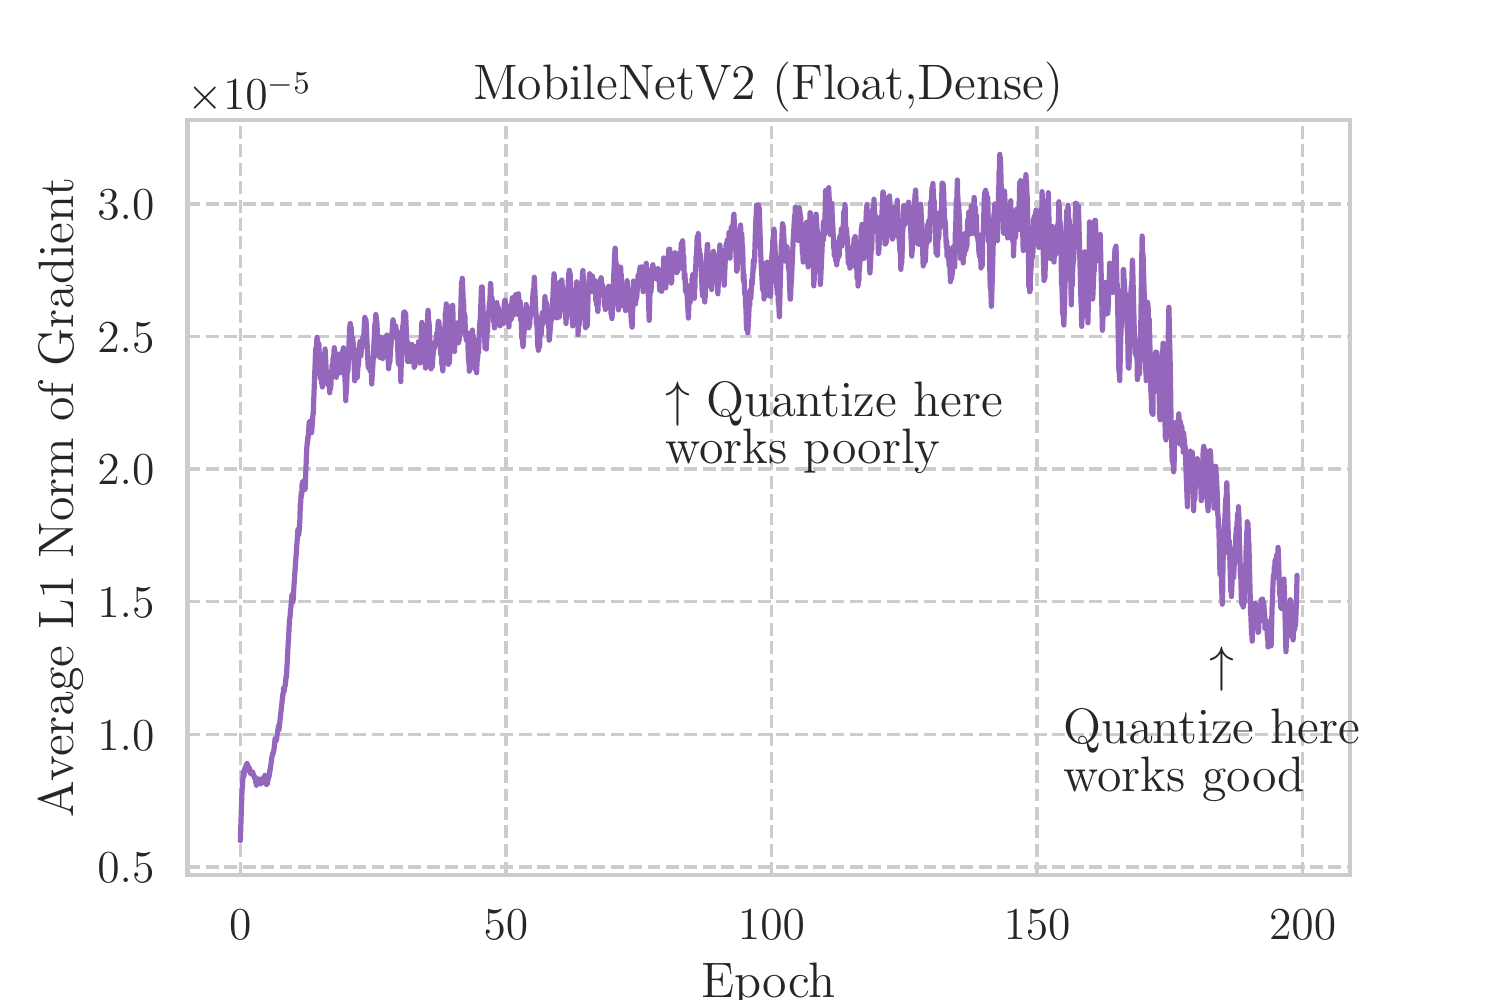}
		}
	\end{center}
	\caption{Visual explanation of why quantizing only works for CIFAR10 
	when applying during late stage of the training process.}
	\label{fig:why_quantize_later}
\end{figure}


% \begin{wraptable}[5]{l}{17em}
\begin{table}[]
	\begin{tabular}{|l|l|}
		\hline
		\textbf{ResNet101}                                 & \textbf{mAP} \\ \hline
		Baseline                                    & 74.47        \\ \hline
		\begin{tabular}[c]{@{}l@{}} {\footnotesize\pq{w,f}{w,f}, $b_f = 32$}    \end{tabular} & 73 (-1.47)   \\ \hline
		{\footnotesize\pq{w,f}{w,f}, $b_f = 1$  }                     & 72.6 (-1.87) \\ \hline
	\end{tabular}
	\caption{Results of quantized and pruned Faster RCNN on Pascal VOC 2007 test
	set with different buffer size $b_f$. \todo{\scriptsize change to plots and add more
	choices of $b_f$}}
	\label{tb:frcnn_bf}
\end{table}
% \end{wraptable}	




\section{Software Interface}
\label{apn:software}

\begin{listing}[]
	\python{snippets/interface.py}
	\caption{Examples to demonstrate our software interface for quantization and pruning}
	\label{code:interface}
\end{listing}


\section{More Samples from Pix2Pix and CycleGAN}
\label{apn:more_demos}
